# Supplementary material for: Adversarial Attacks are Reversible with Natural Supervision
Source: arXiv:2103.14222 source file (2021-09-09)
Supplement: Supplementary file 2 [file theory.tex]

\section{Proof for Theoretical Analysis}
